# Supplementary material for: Raising the Bar in Graph OOD Generalization: Invariant Learning Beyond Explicit Environment Modeling
Source: arXiv:2502.10706 source file (2025-08-02)
Supplement: Supplementary file 1 [file ablation.tex]

\begin{wraptable}{r}{0.55\textwidth}
    \vspace{-8mm}
    \begin{minipage}{0.55\textwidth}
\caption{Performance of \ourmethod and its variants.} 
\resizebox{1\columnwidth}{!}{
  \begin{tabular}{l|ccc}
    \toprule
    \textbf{Variants} &\textbf{CMNIST-color} &\textbf{HIV-scaffold} &\textbf{IC50-size} \\
    \midrule
\ourmethod & \textbf{41.29 (3.85)} & \textbf{74.69 (1.77)} & \textbf{68.06 (0.55)}  \\
    ERM & 26.64 (2.37) & 69.55 (2.39) & 66.10 (0.31)  \\
\midrule
w/o $\mathcal{L}_\textrm{IPM}$ & 37.86 (3.44) & 70.61 (1.52) & 67.09 (0.65)  \\
w/o $\mathcal{L}_\textrm{PS}$ & 37.53 (2.18) & 71.06 (1.56) & 66.21 (0.37) \\
\midrule
w/o Project & 21.05 (4.89) & 65.78 (3.57) & 51.96 (2.54) \\
w/o Multi-P & 20.58 (3.78) & 62.11 (1.95) & 57.64 (1.02)  \\
w/o {Inv. Enc.} & 34.86 (2.92) & 66.72 (1.19) & 63.73 (0.89)  \\
\midrule
w/o Update & 38.95 (3.01) & 67.89 (1.84) & 64.14 (1.22)  \\
w/o Prune & 40.58 (3.78) & 71.11 (1.95) & 67.64 (1.02) \\
    \bottomrule
  \end{tabular}}\label{tab:ablation}
    \end{minipage}
    \vspace{-2mm}
\end{wraptable}
