# Supplementary material for: Raising the Bar in Graph OOD Generalization: Invariant Learning Beyond Explicit Environment Modeling
Source: arXiv:2502.10706 source file (2025-08-02)
Supplement: Supplementary file 2 [file main.tex]

\begin{table*}[t]
\caption{Performance comparison in terms of accuracy. Detailed results with standard deviation are in Table~\ref{tab:main_good} and \ref{tab:main_drugood}. The best and runner-up results are highlighted in \textbf{bold} and \underline{underlined}. The results of MoleOOD/iMoLD on Motif/CMNIST are not available since they are molecule-specific methods.}
\centering
\resizebox{1\textwidth}{!}{
\begin{tabular}{l|cc|c|cc|ccc|ccc}
\toprule
\multirow{3}{*}{\textbf{Method}} & \multicolumn{5}{c|}{\textbf{GOOD}} & \multicolumn{6}{c}{\textbf{DrugOOD}} \\
 & \multicolumn{2}{c|}{\textbf{Motif}} & \textbf{CMNIST} & \multicolumn{2}{c|}{\textbf{HIV}} & \multicolumn{3}{c|}{\textbf{IC50}} & \multicolumn{3}{c}{\textbf{EC50}} \\
 & \textbf{basis} & \textbf{size} & \textbf{color} & \textbf{scaffold} & \textbf{size} & \textbf{assay} & \textbf{scaffold} & \textbf{size} & \textbf{assay} & \textbf{scaffold} & \textbf{size} \\
\midrule
ERM & 60.93  & 46.63  & 26.64  & 69.55  & 59.19  & 70.61  & 67.54  & 66.10  & 65.27  & 65.02  & 65.17  \\
IRM & 64.94  & 54.52  & 29.63  & 70.17  & 59.94  & 71.15  & 67.22  & \underline{67.58} & 67.77  & 63.86  & 59.19  \\
VREX & 61.59  & \underline{55.85} & 27.13  & 69.34  & 58.49  & 70.98  & 68.02  & 65.67  & 69.84  & 62.31  & 65.89 \\
Coral & 61.95  & 55.80  & 29.21  & 70.69  & 59.39  & 71.28  & 68.36  & 67.53  & 72.08  & 64.83  & 58.47  \\
\midrule
MoleOOD & - & - & - & 69.39  & 58.63  & 71.62  & 68.58  & 67.22  & 72.69  & 65.78  & 64.11  \\
CIGA & 67.81  & 51.87  & 25.06  & 69.40  & 61.81 & \underline{71.86} & \textbf{69.14} & 66.99  & 69.15  & 67.32 & 65.60  \\
GIL & 65.30  & 54.65  & 31.82  & 68.59  & 60.97  & 70.66  & 67.81  & 66.23  & 70.25  & 63.95  & 64.91  \\
GREA & 59.91  & 47.36  & 22.12  & 71.98 & 60.11  & 70.23  & 67.20  & 66.09  & 74.17  & 65.84  & 61.11 \\
IGM & \underline{74.69} & 52.01  & 33.95  & 71.36 & 62.54  & 68.05  & 63.16  & 63.89  & 76.28  & \underline{67.57}  & 60.98\\
\midrule
DIR & 64.39  & 43.11  & 22.53  & 68.44  & 57.67  & 69.84  & 66.33  & 62.92  & 65.81  & 63.76  & 61.56  \\
DisC & 65.08  & 42.23  & 23.53  & 58.85  & 49.33  & 61.40  & 62.70  & 64.43  & 63.71  & 60.57  & 57.38  \\
\midrule
GSAT & 62.27  & 50.03  & \underline{35.02} & 70.07  & 60.73  & 70.59  & 66.94  & 64.53  & 73.82  & 62.65  & 62.65  \\
CAL & 68.01 & 47.23  & 27.15  & 69.12  & 59.34  & 70.09  & 65.90  & 64.42  & 74.54 & 65.19  & 61.21  \\
iMoLD & - & -  & -  & {72.05}  & {62.86}  & 71.77  & 67.94  & 66.29  & {77.23} & 66.95  & \underline{67.18}  \\
\textcolor{black}{GALA} & \textcolor{black}{72.97} & \textcolor{black}{\textbf{60.82}} & \textcolor{black}{\underline{40.62}} & \textcolor{black}{71.22}& \textcolor{black}{\underline{65.29}}  & \textcolor{black}{70.58} & \textcolor{black}{66.35} & \textcolor{black}{66.54}  & \textcolor{black}{{77.24}} & \textcolor{black}{66.98} & \textcolor{black}{63.71} \\
\textcolor{black}{EQuAD}      &\textcolor{black}{\underline{75.46}}   & \textcolor{black}{55.10}   & \textcolor{black}{{40.29}}   & \textcolor{black}{71.49}    &\textcolor{black}{{64.09}}  &\textcolor{black}{71.57} & \textcolor{black}{67.74} & \textcolor{black}{67.54} &\textcolor{black}{\underline{77.64}} &\textcolor{black}{65.73} &\textcolor{black}{64.39}  \\
\midrule
\ourmethod & \textbf{76.23} & {58.43} & \textbf{41.29} & \textbf{74.69} & \textbf{66.84} & \textbf{72.96} & \underline{68.62} & \textbf{68.06} & \textbf{78.08} & \textbf{68.94} & \textbf{68.11} \\
\bottomrule
\end{tabular}
}\label{tab:main}
\vspace{-5mm}
\end{table*}
